# Supplementary material for: CADDeLaG: Framework for distributed anomaly detection in large dense graph sequences
Source: arXiv:1802.05421 source file (2018-02-15)
Supplement: Supplementary file 1 [file appendix.tex]

\clearpage

\section{Appendix}

\textbf{Definitions}

$A_k  = D_0 (D_0 A_0) ^{2^k} $, \qquad $S_0  = D^{-1/2}_0 A_0 D^{-1/2}_0 $

\begin{align*}
A_k  &= A_{k-1} D^{-1}_0 A_{k-1}. \\ 
S^2_0  &= D^{-1/2}_0 A_0 D^{-1/2}_0  D^{-1/2}_0 A_0 D^{-1/2}_0 \\ 
&=  D^{-1/2}_0 (A_0 D^{-1}_0 A_0) D^{-1/2}_0 \\ 
&= D^{-1/2}_0 A_1 D^{-1/2}_0 \\
S^3_0  &= D^{-1/2}_0 A_2 D^{-1/2}_0 \\
\cdots \\
S^d_0  &= D^{-1/2}_0 A_{d-1} D^{-1/2}_0 \\
\end{align*}

\begin{figure}[!htb]
\centering
    \includegraphics[width=1.1\linewidth]{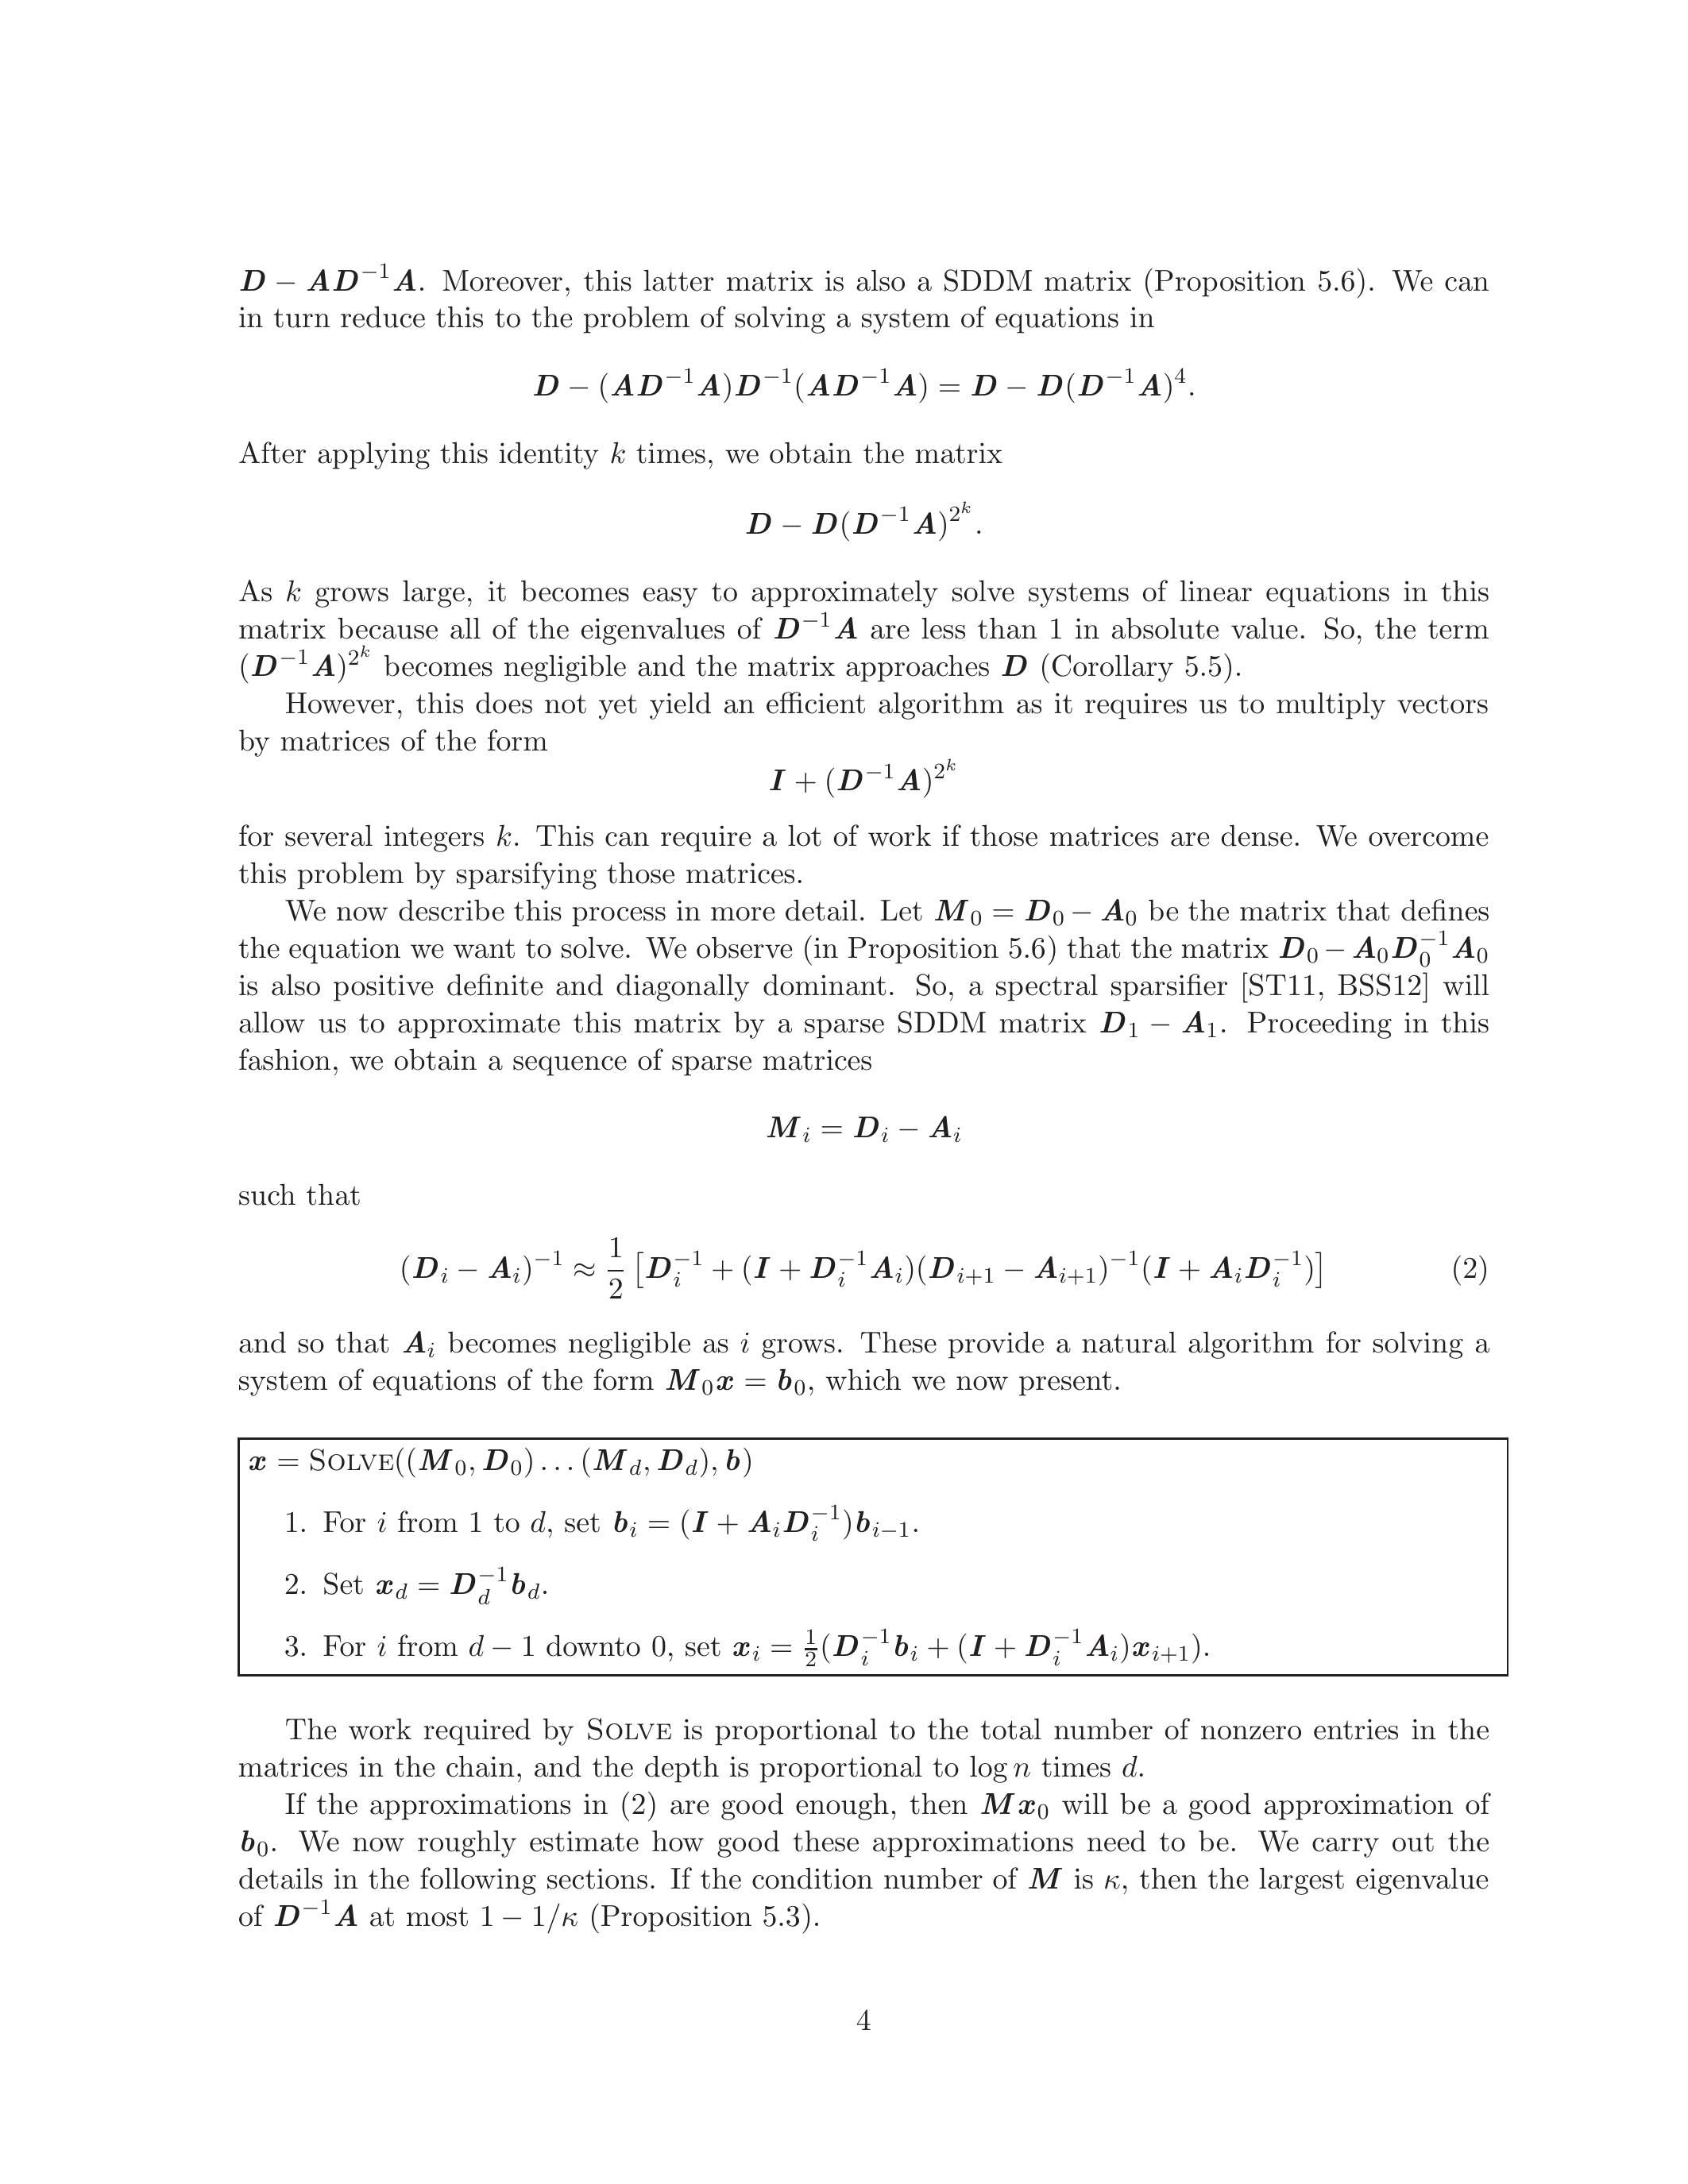}
 \caption{Crude solver algorithm from Spielman Peng paper.}
    \label{fig:cude-solver}
\end{figure}

\begin{align*}
x_{d} &= D^{-1}_d b_{d} = D^{-1/2} I D^{-1/2} b_{d}\\
x_{d-1} &= \frac{1}{2} \big[ D^{-1}_{d-1} b_{d-1} + (I + D^{-1}_{d-1}A_{d-1})x_{d} \big] \\
        &= \frac{1}{2} \big[ D^{-1}_{d-1} b_{d-1} + (I + D^{-1}_{d-1}A_{d-1})D^{-1}_d b_{d} \big] \\
        &= \frac{1}{2} \big[ D^{-1} b_{d-1} + (I + D^{-1}A_{d-1})D^{-1} (I + A_{d-1} D^{-1}) b_{d-1} \big] \\
        &= \frac{1}{2} \big[ D^{-1} + (I + D^{-1}A_{d-1}) (D^{-1} + D^{-1} A_{d-1} D^{-1}) \big] b_{d-1} \\
        &= \frac{1}{2} \big[ D^{-1} + D^{-1} + D^{-1} A_{d-1} D^{-1} + D^{-1} A_{d-1} D^{-1} + D^{-1} A_{d-1} D^{-1} A_{d-1} D^{-1} \big] b_{d-1} \\
        &= \big[ D^{-1} + D^{-1} A_{d-1} D^{-1} + \frac{1}{2} D^{-1} A_{d} D^{-1} \big] b_{d-1} \\
        &= \big[ D^{-1} + D^{-1/2} S^d_{0} D^{-1/2} + \frac{1}{2} D^{-1/2} S^{d+1}_0 D^{-1/2} \big] b_{d-1} \\
        &= D^{-1/2} \big[I + S^d_{0} + \frac{1}{2} S^{d+1}_0 \big] D^{-1/2} b_{d-1} \\
        .
        % &= \frac{1}{2} \big[ D^{-1}_{d-1} b_{d-1} + (I + D^{-1}_{d-1}A_{d-1})x_{d} \big] \\
        % &= \frac{1}{2} \big[ D^{-1}_{d-1} b_{d-1} + (I + D^{-1}_{d-1}A_{d-1})x_{d} \big] \\
\end{align*}

\clearpage
\newpage

 \begin{algorithm}
 \SetAlgoLined
    \SetKwInOut{Input}{Input}
    \SetKwInOut{Output}{Output}
    \Input{$D, A, b, d$}
    \Output{Crude approximation, $\hat{x}$, of $M^{-1}b$}
    $C = D^{-1/2} b$ \\
    $S = D^{-1/2} A D^{-1/2}$ \\
    $y = (I+S)(I+S^2)\cdots(I+S^{2^{d-1}})C$ \\
    return  $y$\;
    \caption{CrudeSolve}
    \label{alg:crude-solve}
\end{algorithm}
 \begin{algorithm}
 \SetAlgoLined
    \SetKwInOut{Input}{Input}
    \SetKwInOut{Output}{Output}
    \Input{$D, A, b, d, \delta$}
    \Output{ $\delta$ close approximation, $x^*$, of $M^{-1}b$}
    $q = \left \lceil \log(1/\delta) \right \rceil$ \\
    $\hat{x} =$  CrudeSolve$(D, A, b, d)$ \\
    $\chi = D^{-1/2} \hat{x} $\\
    // Preconditioned Richardson iterative scheme\\
    $y_1 = 0$ \\
    For $k = 1 $ to $q-1$ \\
    \quad $u_k = (D - A)y_k$ \\
    \quad $\hat{x} =$  CrudeSolve$(D, A, u_k, d)$ \\
    \quad $u^2_k = D^{-1/2} \hat{x}$ \\
    \quad $y_{k+1} = y_k - u^2_k + \chi$ \\
    return $y_q$
    \caption{ExactSolve}
    \label{alg:exact-solve}
\end{algorithm}

\begin{algorithm}
 \SetAlgoLined
    \SetKwInOut{Input}{Input}
    \SetKwInOut{Output}{Output}
    \Input{$D, A, d$}
    \Output{Preprocessing for crude approximation, $\bar{\mathbf{P}}_1, \bar{\mathbf{P}}_2$}
    $S = D^{-1/2} A D^{-1/2}$ \\
    $\mathbf{P} = (I+S)(I+S^2)\cdots(I+S^{2^{d-1}})\mathbf{C}$ \\
    $\bar{\mathbf{P}}_1, \bar{\mathbf{P}}_2 = D^{-1/2} \mathbf{P}, D^{-1/2} \mathbf{P} L $  \\  
    \caption{PreCrudeSolver}
    \label{alg:pre-crude-solve}
\end{algorithm}

\begin{algorithm}
 \SetAlgoLined
    \SetKwInOut{Input}{Input}
    \SetKwInOut{Output}{Output}
    \Input{$\bar{\mathbf{P}}_1, \bar{\mathbf{P}}_2, y, \delta$}
    \Output{ $\delta$ close approximation, $x*$, of $M^{-1}b$}
    $q = \left \lceil \log(1/\delta) \right \rceil$ \\
    $\chi = \bar{\mathbf{P}}_1 y$\\
    $y_1 = 0$ \\
    For $k = 1 $ to $q-1$ \\
    \quad $y_{k+1} = y_k - \bar{\mathbf{P}}_2 y_k + \chi$ \\
    return $y_q$
    \caption{ExactSolveFast}
    \label{alg:exact-solve-new}
\end{algorithm}

\begin{algorithm}
 \SetAlgoLined
    \SetKwInOut{Input}{Input}
    \SetKwInOut{Output}{Output}
    \Input{$\bar{\mathbf{P}}_1, \bar{\mathbf{P}}_2, y, \delta$}
    \Output{ $\delta$ close approximation, $x*$, of $M^{-1}b$}
    $q = \left \lceil \log(1/\delta) \right \rceil$ \\
    $\chi = \bar{\mathbf{P}}_1 y$\\
    $y_1 = \chi$ \\
    For $k = 1 $ to $q-2$ \\
    \quad $y_{k+1} = y_k - \bar{\mathbf{P}}_2 y_k + \chi$ \\
    return $y_{q-1}$
    \caption{ExactSolveFast2}
    \label{alg:exact-solve-new}
\end{algorithm}

\begin{algorithm}
 \SetAlgoLined
    \SetKwInOut{Input}{Input}
    \SetKwInOut{Output}{Output}
    \Input{$G, E, \epsilon_{RP}, \delta$}
    \Output{ $\epsilon_{RP}$ close approximations, $d_{ij}$, of commute time distances between $(i,j)$ for all $(i,j) \in E$}
    $D^{G} \leftarrow $ Diagonal matrix with row-sums of $G$ as the elements\\
    $L = D^{G} - G$ \\
    Compute $B, W $ according to Equation~\ref{eq:def-B}\\
    $C = \{ d_{ij}  | (i,j) \in E \}$ \\
    $C  \leftarrow 0 $ \\
    $n \leftarrow $ Number of nodes in $G$ \\ 
    $k_{RP} = \left \lceil \log(n/\epsilon_{RP}) \right \rceil$ \\
    %     
%     \\
    // ----- Chain computation --- \\
    $\mathbf{C}_1 = D^{-1/2} $ \\
    $S = D^{-1/2} G D^{-1/2}$ \\
    $\mathbf{P} = (I+S)(I+S^2)\cdots(I+S^{2^{d-1}})\mathbf{C}_1$ \\
    $\bar{\mathbf{P}}_1 = D^{-1/2} \mathbf{P} $ \\
    $\bar{\mathbf{P}}_2 = \bar{\mathbf{P}}_1 L $  \\  
    // -------------------------- \\  
%      \\
    For $j = 1 $ to $k_{RP}$ \\
    Create random vector $q$ \\
     $y = W^{1/2} B q$ \\
     $z = $ ExactSolveFast$(\bar{\mathbf{P}}_1, \bar{\mathbf{P}}_2, y, \delta)$ \\
     $\forall (i,j) \in E$, do: \\
    \qquad $d_{ij}  \leftarrow d_{ij} + (z_i - z_j)^2 $ \\
    return C
    \caption{CommuteTimeDistancesFast}
    \label{alg:commute-time-dist-refactored}
\end{algorithm}

\begin{algorithm}
 \SetAlgoLined
    \SetKwInOut{Input}{Input}
    \SetKwInOut{Output}{Output}
    \Input{$G, E, \epsilon_{RP}, \delta$}
    \Output{ Embedding $Z$ for $\epsilon_{RP}$ close approximations, $d_{ij}$}
    $D^{G} \leftarrow $ Diagonal matrix: row-sums of $G$ \\
    $L = D^{G} - G$ \\
    Compute $B, W $ according to Equation~\ref{eq:def-B}\\
    $n \leftarrow $ Number of nodes in $G$ \\ 
    $k_{RP} = \left \lceil \log(n/\epsilon_{RP}) \right \rceil$ \\
    $q = \left \lceil \log(1/\delta) \right \rceil$ \\
%     \\
    // ----- Chain computation --- \\
    $S = D^{-1/2} G D^{-1/2}$ \\
    $\mathbf{P} = (I+S)(I+S^2)\cdots(I+S^{2^{d-1}}) D^{-1/2}$ \\
    $\bar{\mathbf{P}}_1, \bar{\mathbf{P}}_2 = D^{-1/2} \mathbf{P}, D^{-1/2} \mathbf{P} L $  \\  
    // -------------------------- \\  
%      \\
    For $j = 1 $ to $k_{RP}$ \\
    Create random vector $\eta$ \\
     $y = W^{1/2} B \eta$ \\    
     $\chi = \bar{\mathbf{P}}_1 y$\\
     $y_1 = \chi$ \\
     For $k = 1 $ to $q-2$ \\
     \quad $y_{k+1} = y_k - \bar{\mathbf{P}}_2 y_k + \chi$ \\
     $Z_i = y_{q-1}$

    return $Z$
    \caption{CommuteTimeEmbeddingFast}
    \label{alg:commute-time-dist-refactored}
\end{algorithm}
